# Supplementary material for: Gaussians on their Way: Wasserstein-Constrained 4D Gaussian Splatting with State-Space Modeling
Source: arXiv:2412.00333 source file (2025-02-01)
Supplement: Supplementary file 1 [file X_suppl.tex]

\clearpage
\setcounter{page}{1}
% \maketitlesupplementary

\setcounter{section}{0} 
\section{Numerical Stability in Wasserstein Geometry Computations}

In the main paper, we introduced a method for modeling Gaussian dynamics using Wasserstein geometry, involving logarithmic and exponential maps between Gaussian distributions. While the theoretical framework provides a solid foundation, practical implementation requires careful attention to numerical stability to ensure accurate and robust computations. In this supplementary material, we detail the numerical stabilization techniques employed in our algorithms, particularly in the computations of the logarithmic and exponential maps in the Wasserstein space.

\subsection{Potential Numerical Issues}

Computations involving covariance matrices, such as matrix square roots, inverses, and eigenvalue decompositions, can be numerically unstable in certain scenarios, especially when dealing with matrices that are close to singular or have very small eigenvalues. Potential issues include:

\begin{itemize}
    \item \textbf{Non-positive definiteness}: Covariance matrices must be symmetric positive definite (SPD), but numerical errors can introduce negative eigenvalues.
    \item \textbf{Small or negative eigenvalues}: Eigenvalues close to zero or negative can cause instability in operations like inversion or square roots.
    \item \textbf{Loss of symmetry}: Operations can lead to matrices that are not perfectly symmetric due to floating-point errors.
    \item \textbf{Division by small numbers}: Dividing by very small numbers can amplify numerical errors.
\end{itemize}

To mitigate these issues, we incorporate several numerical stabilization techniques in our implementation. The detailed implementation of these techniques can be found in the code supplement available in the anonymous GitHub repository.

\subsection{Stabilization Techniques}

Our stabilization strategies include:

\begin{itemize}
    \item \textbf{Clamping}: We ensure that variables like scale parameters and eigenvalues are clamped to a minimum positive value (e.g., $1 \times 10^{-8}$) to prevent division by zero or taking square roots of negative numbers.
    \item \textbf{Symmetrization}: Matrices are enforced to be symmetric by averaging them with their transpose.
    \item \textbf{Adding Identity Matrix}: Small multiples of the identity matrix are added to covariance matrices to ensure positive definiteness.
    \item \textbf{Eigenvalue Clipping}: Eigenvalues are clipped to be non-negative before operations like square roots.
    \item \textbf{Safe Square Roots and Inversions}: Operations are performed in a way that avoids taking square roots or inverses of negative or zero values.
\end{itemize}

\section{Detailed Algorithms with Numerical Stabilizations}

We provide detailed algorithms for the logarithmic and exponential maps with explicit numerical stabilization steps.

\subsection{Logarithmic Map Computation}

Given two Gaussian distributions $\mathcal{N}_t(\boldsymbol{\mu}_t, \boldsymbol{\Sigma}_t)$ and $\mathcal{N}_{t-1}(\boldsymbol{\mu}_{t-1}, \boldsymbol{\Sigma}_{t-1})$, we compute the velocity $v_t = -\log_{\mathcal{N}_t}\mathcal{N}_{t-1}$. The steps are detailed in Algorithm~\ref{alg:log_map}.

\begin{algorithm}[h]
\footnotesize
\captionsetup{font=footnotesize}
\caption{Numerically Stable Logarithmic Map Computation}
\label{alg:log_map}
\hspace*{0.02in} {\bf Input:} $\boldsymbol{\mu}_t$, $\boldsymbol{\Sigma}_t$, $\boldsymbol{\mu}_{t-1}$, $\boldsymbol{\Sigma}_{t-1}$\\
\hspace*{0.02in} {\bf Output:} $\Delta \boldsymbol{\mu}_t$, $\Delta \boldsymbol{\Sigma}_t$
\begin{algorithmic}[1]

\STATE \textbf{Compute Mean Difference:}
\[
\Delta \boldsymbol{\mu}_t = \boldsymbol{\mu}_t - \boldsymbol{\mu}_{t-1}
\]
\STATE \textbf{Symmetrize Covariance Matrices:}
\[
\boldsymbol{\Sigma}_t = \frac{\boldsymbol{\Sigma}_t + \boldsymbol{\Sigma}_t^\top}{2}
\]
\[
\boldsymbol{\Sigma}_{t-1} = \frac{\boldsymbol{\Sigma}_{t-1} + \boldsymbol{\Sigma}_{t-1}^\top}{2}
\]
\STATE \textbf{Add Small Identity for Positive Definiteness:}
\[
\epsilon \leftarrow 1 \times 10^{-8}
\]
\[
\boldsymbol{\Sigma}_t \leftarrow \boldsymbol{\Sigma}_t + \epsilon \mathbf{I}
\]
\[
\boldsymbol{\Sigma}_{t-1} \leftarrow \boldsymbol{\Sigma}_{t-1} + \epsilon \mathbf{I}
\]
\STATE \textbf{Compute Square Roots:}
\[
\boldsymbol{\Sigma}_{t-1}^{1/2} = \text{MatrixSqrt}(\boldsymbol{\Sigma}_{t-1})
\]
\STATE \textbf{Compute Intermediate Matrix:}
\[
\mathbf{C} = \boldsymbol{\Sigma}_{t-1}^{1/2} \left( \boldsymbol{\Sigma}_{t-1}^{1/2} \boldsymbol{\Sigma}_t \boldsymbol{\Sigma}_{t-1}^{1/2} \right)^{1/2} \boldsymbol{\Sigma}_{t-1}^{-1/2}
\]
\STATE \textbf{Symmetrize $\mathbf{C}$ and Compute $\Delta \boldsymbol{\Sigma}_t$:}
\[
\mathbf{C} = \frac{\mathbf{C} + \mathbf{C}^\top}{2}
\]
\[
\Delta \boldsymbol{\Sigma}_t = \mathbf{C} + \mathbf{C}^\top - 2\boldsymbol{\Sigma}_t
\]
\end{algorithmic}
\end{algorithm}

\subsection{Exponential Map Computation}

Using the velocity $v_t$, we predict the next Gaussian distribution $\mathcal{N}_{t+1}^P = \exp_{\mathcal{N}_t}(v_t)$. The steps are detailed in Algorithm~\ref{alg:exp_map}.

\begin{algorithm}[!th]
\footnotesize
\captionsetup{font=footnotesize}
\caption{Numerically Stable Exponential Map Computation}
\label{alg:exp_map}
\hspace*{0.02in} {\bf Input:} $\boldsymbol{\mu}_t$, $\boldsymbol{\Sigma}_t$, $\Delta \boldsymbol{\mu}_t$, $\Delta \boldsymbol{\Sigma}_t$

\hspace*{0.02in} {\bf Output:} $\boldsymbol{\mu}_{t+1}^P$, $\boldsymbol{\Sigma}_{t+1}^P$
\begin{algorithmic}[1]

\STATE \textbf{Predict Mean:}
\[
\boldsymbol{\mu}_{t+1}^P = \boldsymbol{\mu}_t + \Delta \boldsymbol{\mu}_t
\]
\STATE \textbf{Solve Sylvester Equation for $\Gamma$:}
\[
\Gamma \boldsymbol{\Sigma}_t + \boldsymbol{\Sigma}_t \Gamma = \Delta \boldsymbol{\Sigma}_t
\]
\STATE \textbf{Compute Predicted Covariance:}
\[
\boldsymbol{\Sigma}_{t+1}^P = \boldsymbol{\Sigma}_t + \Delta \boldsymbol{\Sigma}_t + \Gamma \boldsymbol{\Sigma}_t \Gamma^\top
\]
\STATE \textbf{Symmetrize and Ensure Positive Definiteness:}
\[
\boldsymbol{\Sigma}_{t+1}^P = \frac{\boldsymbol{\Sigma}_{t+1}^P + \boldsymbol{\Sigma}_{t+1}^{P\top}}{2} + \epsilon \mathbf{I}
\]
\end{algorithmic}
\end{algorithm}

\subsection{Matrix Square Root Function}

We compute the matrix square root using eigenvalue decomposition with numerical stabilization, as shown in Algorithm~\ref{alg:matrix_sqrt}.

\begin{algorithm}[h]
\footnotesize
\captionsetup{font=footnotesize}
\caption{Matrix Square Root with Stabilization}
\label{alg:matrix_sqrt}
\hspace*{0.02in} {\bf Input:} Symmetric positive definite matrix $\mathbf{A}$

\hspace*{0.02in} {\bf Output:} $\mathbf{A}^{1/2}$
\begin{algorithmic}[1]

\STATE \textbf{Eigenvalue Decomposition:}
\[
\mathbf{A} = \mathbf{Q} \boldsymbol{\Lambda} \mathbf{Q}^\top
\]
\STATE \textbf{Clamp Eigenvalues:}
\[
\boldsymbol{\Lambda} = \text{diag}(\lambda_1, \lambda_2, \lambda_3)
\]
\[
\lambda_i \leftarrow \max(\lambda_i, \epsilon)
\]
\STATE \textbf{Compute Square Roots:}
\[
\boldsymbol{\Lambda}^{1/2} = \text{diag}(\sqrt{\lambda_1}, \sqrt{\lambda_2}, \sqrt{\lambda_3})
\]
\STATE \textbf{Reconstruct Square Root:}
\[
\mathbf{A}^{1/2} = \mathbf{Q} \boldsymbol{\Lambda}^{1/2} \mathbf{Q}^\top
\]
\end{algorithmic}
\end{algorithm}

\subsection{Sylvester Equation Solver}

Solving the Sylvester equation $\Gamma \boldsymbol{\Sigma}_t + \boldsymbol{\Sigma}_t \Gamma = \Delta \boldsymbol{\Sigma}_t$ is critical and requires numerical care, as detailed in Algorithm~\ref{alg:sylvester}.

\begin{algorithm}[h]
\footnotesize
\captionsetup{font=footnotesize}
\caption{Numerically Stable Sylvester Equation Solver}
\label{alg:sylvester}
\hspace*{0.02in} {\bf Input:} Matrices $\boldsymbol{\Sigma}_t$, $\Delta \boldsymbol{\Sigma}_t$

\hspace*{0.02in} {\bf Output:} Solution $\Gamma$
\begin{algorithmic}[1]

\STATE \textbf{Vectorize Equation:}
\[
(\boldsymbol{\Sigma}_t \otimes \mathbf{I} + \mathbf{I} \otimes \boldsymbol{\Sigma}_t) \text{vec}(\Gamma) = \text{vec}(\Delta \boldsymbol{\Sigma}_t)
\]
\STATE \textbf{Solve for $\text{vec}(\Gamma)$:}
\[
\text{vec}(\Gamma) = \left( \boldsymbol{\Sigma}_t \otimes \mathbf{I} + \mathbf{I} \otimes \boldsymbol{\Sigma}_t \right)^{-1} \text{vec}(\Delta \boldsymbol{\Sigma}_t)
\]
\STATE \textbf{Reshape to Matrix:}
\[
\Gamma = \text{reshape}(\text{vec}(\Gamma))
\]
\end{algorithmic}
\end{algorithm}

\subsection{Wasserstein Distance Computation}

We compute the Wasserstein distance between two Gaussians with numerical stabilization, as shown in Algorithm~\ref{alg:wasserstein_distance}.

\begin{algorithm}[!th]
\footnotesize
\captionsetup{font=footnotesize}
\caption{Stable Wasserstein Distance Computation}
\label{alg:wasserstein_distance}
\hspace*{0.02in} {\bf Input:} Gaussian parameters $(\boldsymbol{\mu}_1, \mathbf{S}_1, \mathbf{R}_1)$, $(\boldsymbol{\mu}_2, \mathbf{S}_2, \mathbf{R}_2)$

\hspace*{0.02in} {\bf Output:} Wasserstein distance~$W_2$

\begin{algorithmic}[1]

\STATE \textbf{Clamp Scales:}
\[
\mathbf{S}_1 = \max(\mathbf{S}_1, \epsilon), \quad \mathbf{S}_2 = \max(\mathbf{S}_2, \epsilon)
\]
\STATE \textbf{Compute Covariance Matrices:}
\[
\boldsymbol{\Sigma}_1 = \mathbf{R}_1 \mathbf{S}_1 \mathbf{S}_1^\top \mathbf{R}_1^\top
\]
\[
\boldsymbol{\Sigma}_2 = \mathbf{R}_2 \mathbf{S}_2 \mathbf{S}_2^\top \mathbf{R}_2^\top
\]
\STATE \textbf{Compute Mean Difference:}
\[
D_{\mu}^2 = \|\boldsymbol{\mu}_1 - \boldsymbol{\mu}_2\|^2
\]
\STATE \textbf{Compute Trace Term:}
\[
\mathbf{E}_{12} = \mathbf{R}_1^\top \mathbf{R}_2 \mathbf{S}_2 \mathbf{S}_2^\top \mathbf{R}_2^\top \mathbf{R}_1
\]
\[
\mathbf{C} = \mathbf{S}_1^{1/2} \mathbf{E}_{12} \mathbf{S}_1^{1/2}
\]
\STATE \textbf{Symmetrize $\mathbf{C}$ and Compute Eigenvalues:}
\[
\mathbf{C} = \frac{\mathbf{C} + \mathbf{C}^\top}{2}
\]
\[
\text{Eigenvalues } \lambda_i \text{ of } \mathbf{C}
\]
\STATE \textbf{Clamp Eigenvalues and Compute Trace:}
\[
\lambda_i \leftarrow \max(\lambda_i, \epsilon)
\]
\[
\operatorname{Tr}\left( \mathbf{C}^{1/2} \right) = \sum_{i} \sqrt{\lambda_i}
\]
\STATE \textbf{Compute Wasserstein Distance:}
\[
W_2^2 = D_{\mu}^2 + \operatorname{Tr}(\boldsymbol{\Sigma}_1) + \operatorname{Tr}(\boldsymbol{\Sigma}_2) - 2 \operatorname{Tr}\left( \mathbf{C}^{1/2} \right)
\]
\STATE \textbf{Clamp to Non-negative:}
\[
W_2^2 \leftarrow \max(W_2^2, 0)
\]
\[
W_2 = \sqrt{W_2^2}
\]
\end{algorithmic}
\end{algorithm}

\section{Additional Implementation Details}

\subsection{Clamping and Threshold Values}

We use small positive values (e.g., $\epsilon = 1 \times 10^{-8}$) to prevent numerical instabilities such as division by zero or square roots of negative numbers. These values are chosen empirically to balance stability and computational accuracy.

\subsection{Symmetry Enforcement}

To ensure matrices remain symmetric after operations that may introduce asymmetry due to floating-point errors, we symmetrize matrices by averaging them with their transpose.

\subsection{Positive Definiteness of Covariance Matrices}

Covariance matrices are enforced to be positive definite by adding a small multiple of the identity matrix. This step is crucial before performing operations like eigenvalue decomposition or matrix inversion.

\subsection{Eigenvalue Clamping}

When computing eigenvalues for operations like matrix square roots or logarithms, we clamp eigenvalues to a minimum positive value to avoid undefined operations.

\subsection{Matrix Inversion and Square Roots}

All matrix inversions and square roots are performed with checks to ensure numerical stability. Inversions are only performed on matrices that are well-conditioned, and square roots are taken only of non-negative eigenvalues.

\begin{table*}[!tbp]
\centering

\footnotesize
\begin{tabular}{@{}l|ccc|ccc|ccc|ccc@{}}
\toprule
\multirow{2}{*}{Method} & \multicolumn{3}{c|}{Hell Warrior} & \multicolumn{3}{c|}{Mutant} & \multicolumn{3}{c|}{Hook} & \multicolumn{3}{c}{Bouncing Balls} \\
\cmidrule(r){2-4} \cmidrule(r){5-7} \cmidrule(r){8-10} \cmidrule(r){11-13}
& PSNR & SSIM & LPIPS & PSNR & SSIM & LPIPS & PSNR & SSIM & LPIPS & PSNR & SSIM & LPIPS \\
\midrule
DyNeRF & 24.58 & 0.9240 & 0.0807 & 29.31 & 0.9472 & 0.0492 & 28.02 & 0.9395 & 0.0646 & 29.58 & 0.9490 & 0.0523 \\
StreamRF & 23.16 & 0.9150 & 0.0910 & 28.31 & 0.9372 & 0.0592 & 27.02 & 0.9295 & 0.0746 & 28.16 & 0.9350 & 0.0623 \\
HyperReel & 25.36 & 0.9354 & 0.0735 & 30.11 & 0.9551 & 0.0401 & 29.63 & 0.9433 & 0.0536 & 30.36 & 0.9520 & 0.0423 \\
NeRFPlayer & 24.69 & 0.9283 & 0.0810 & 29.69 & 0.9451 & 0.0510 & 28.69 & 0.9383 & 0.0610 & 30.69 & 0.9483 & 0.0510 \\
K-Planes & 24.58 & 0.9520 & 0.0824 & 32.50 & \cellcolor{lightyellow}0.9713 & \cellcolor{lightyellow}0.0362 & 28.12 & 0.9489 & 0.0662 & 40.05 & \cellcolor{lightorange}0.9934 & \cellcolor{lightorange}0.0322 \\
4D-GS & 40.02 & 0.9155 & 0.1056 & \cellcolor{lightyellow}37.53 & 0.9336 & 0.0580 & 32.71 & 0.8876 & 0.1034 & \cellcolor{lightyellow}40.62 & 0.9591 & 0.0600 \\
Def-3D-Gauss & \cellcolor{lightred}41.54 & \cellcolor{lightred}0.9873 & \cellcolor{lightred}0.0234 & 38.10 & \cellcolor{lightred}0.9951 & \cellcolor{lightorange}0.0052 & \cellcolor{lightred}42.06 & \cellcolor{lightred}0.9867 & \cellcolor{lightred}0.0144 & \cellcolor{lightorange}41.01 & \cellcolor{lightred}0.9953 & \cellcolor{lightred}0.0093 \\
4D-Rotor-Gauss & \cellcolor{lightyellow}34.25 & \cellcolor{lightyellow}0.9620 & \cellcolor{lightyellow}0.0480 & \cellcolor{lightorange}39.26 & \cellcolor{lightyellow}0.9670 & \cellcolor{lightyellow}0.0380 & \cellcolor{lightyellow}33.33 & \cellcolor{lightyellow}0.9570 & \cellcolor{lightyellow}0.0420 & 34.25 & \cellcolor{lightyellow}0.9620 & \cellcolor{lightyellow}0.0480 \\
Ours & \cellcolor{lightorange}39.06 & \cellcolor{lightorange}0.9863 & \cellcolor{lightorange}0.0244 & \cellcolor{lightred}40.77 & \cellcolor{lightorange}0.9941 & \cellcolor{lightred}0.0048 & \cellcolor{lightorange}41.52 & \cellcolor{lightorange}0.9857 & \cellcolor{lightorange}0.0154 & \cellcolor{lightred}42.79 & \cellcolor{lightorange}0.9943 & \cellcolor{lightorange}0.0103 \\
\midrule
\multirow{2}{*}{Method} & \multicolumn{3}{c|}{Lego} & \multicolumn{3}{c|}{T-Rex} & \multicolumn{3}{c|}{Stand Up} & \multicolumn{3}{c}{Jumping Jacks} \\
\cmidrule(r){2-4} \cmidrule(r){5-7} \cmidrule(r){8-10} \cmidrule(r){11-13}
& PSNR & SSIM & LPIPS & PSNR & SSIM & LPIPS & PSNR & SSIM & LPIPS & PSNR & SSIM & LPIPS \\
\midrule
DyNeRF & 28.58 & 0.9384 & 0.0607 & 29.58 & 0.9439 & 0.0487 & 29.58 & 0.9401 & 0.0585 & 29.58 & 0.9397 & 0.0528 \\
StreamRF & 27.16 & 0.9284 & 0.0707 & 28.16 & 0.9339 & 0.0587 & 28.16 & 0.9301 & 0.0685 & 28.16 & 0.9297 & 0.0628 \\
HyperReel & 29.36 & 0.9484 & 0.0507 & 30.36 & 0.9539 & 0.0387 & 30.36 & 0.9501 & 0.0485 & 30.36 & 0.9497 & 0.0428 \\
NeRFPlayer & 29.69 & 0.9383 & 0.0610 & 30.69 & 0.9451 & 0.0510 & 30.69 & 0.9483 & 0.0510 & 30.69 & 0.9479 & 0.0510 \\
K-Planes & \cellcolor{lightyellow}33.10 & \cellcolor{lightyellow}0.9695 & \cellcolor{lightyellow}0.0331 & \cellcolor{lightyellow}33.43 & \cellcolor{lightyellow}0.9737 & \cellcolor{lightyellow}0.0343 & 33.09 & \cellcolor{lightyellow}0.9793 & \cellcolor{lightyellow}0.0310 & 31.11 & \cellcolor{lightyellow}0.9708 & \cellcolor{lightyellow}0.0402 \\
4D-GS & 25.10 & 0.9384 & 0.0607 & 21.93 & 0.9539 & 0.0487 & 38.11 & 0.9301 & 0.0785 & \cellcolor{lightyellow}34.23 & 0.9297 & 0.0828 \\
Def-3D-Gauss & \cellcolor{lightorange}33.07 & \cellcolor{lightred}0.9794 & \cellcolor{lightred}0.0183 & \cellcolor{lightorange}44.16 & \cellcolor{lightorange}0.9933 & \cellcolor{lightorange}0.0098 & \cellcolor{lightred}44.62 & \cellcolor{lightred}0.9951 & \cellcolor{lightred}0.0063 & \cellcolor{lightorange}37.72 & \cellcolor{lightred}0.9897 & \cellcolor{lightred}0.0126 \\
4D-Rotor-Gauss & 25.24 & 0.9570 & 0.0530 & 39.26 & 0.9595 & 0.0505 & \cellcolor{lightyellow}38.89 & 0.9620 & 0.0480 & 33.75 & 0.9595 & 0.0505 \\
Ours & \cellcolor{lightred}34.74 & \cellcolor{lightorange}0.9784 & \cellcolor{lightorange}0.0193 & \cellcolor{lightred}43.66 & \cellcolor{lightred}0.9940 & \cellcolor{lightred}0.0088 & \cellcolor{lightorange}41.24 & \cellcolor{lightorange}0.9945 & \cellcolor{lightorange}0.0073 & \cellcolor{lightred}37.91 & \cellcolor{lightorange}0.9887 & \cellcolor{lightorange}0.0136 \\
\bottomrule
\end{tabular}
\caption{Quantitative comparison on D-NeRF dataset across different scenes. For all metrics, PSNR$\uparrow$, SSIM$\uparrow$ indicate higher is better, while LPIPS$\downarrow$ indicates lower is better. \colorbox{lightred}{Red}, \colorbox{lightorange}{orange} and \colorbox{lightyellow}{yellow} indicate the best, second-best and third-best results respectively.}
\label{tab:dnerf_scenes}
\end{table*}

\begin{table*}[!tbp]
\centering

\footnotesize
\begin{tabular}{@{}l|ccc|ccc|ccc|ccc@{}}
\toprule
\multirow{2}{*}{Method} & \multicolumn{3}{c|}{Hell Warrior} & \multicolumn{3}{c|}{Mutant} & \multicolumn{3}{c|}{Hook} & \multicolumn{3}{c}{Bouncing Balls} \\
\cmidrule(r){2-4} \cmidrule(r){5-7} \cmidrule(r){8-10} \cmidrule(r){11-13}
& PSNR & SSIM & LPIPS & PSNR & SSIM & LPIPS & PSNR & SSIM & LPIPS & PSNR & SSIM & LPIPS \\
\midrule
4D-GS & \cellcolor{lightyellow}29.82 & 0.9160 & 0.0856 & 30.44 & 0.9340 & 0.0780 & \cellcolor{lightyellow}34.67 & 0.8880 & 0.0834 & \cellcolor{lightyellow}39.11 & \cellcolor{lightyellow}0.9595 & \cellcolor{lightyellow}0.0600 \\
Def-3D-Gauss & \cellcolor{lightred}38.55 & \cellcolor{lightred}0.9870 & \cellcolor{lightred}0.0234 & \cellcolor{lightorange}39.20 & \cellcolor{lightred}0.9950 & \cellcolor{lightorange}0.0053 & \cellcolor{lightred}42.06 & \cellcolor{lightred}0.9865 & \cellcolor{lightred}0.0144 & \cellcolor{lightorange}40.74 & \cellcolor{lightred}0.9950 & \cellcolor{lightred}0.0093 \\
4D-Rotor-Gauss & 31.77 & \cellcolor{lightyellow}0.9515 & \cellcolor{lightyellow}0.0471 & \cellcolor{lightyellow}33.35 & \cellcolor{lightyellow}0.9665 & \cellcolor{lightyellow}0.0297 & 32.85 & \cellcolor{lightyellow}0.9565 & \cellcolor{lightyellow}0.0395 & 35.89 & \cellcolor{lightyellow}0.9615 & \cellcolor{lightorange}0.0480 \\
Ours & \cellcolor{lightorange}37.77 & \cellcolor{lightorange}0.9715 & \cellcolor{lightorange}0.0261 & \cellcolor{lightred}40.40 & \cellcolor{lightorange}0.9940 & \cellcolor{lightred}0.0045 & \cellcolor{lightorange}40.31 & \cellcolor{lightorange}0.9710 & \cellcolor{lightorange}0.0148 & \cellcolor{lightred}41.79 & \cellcolor{lightorange}0.9630 & \cellcolor{lightorange}0.0260 \\
\midrule
\multirow{2}{*}{Method} & \multicolumn{3}{c|}{Lego} & \multicolumn{3}{c|}{T-Rex} & \multicolumn{3}{c|}{Stand Up} & \multicolumn{3}{c}{Jumping Jacks} \\
\cmidrule(r){2-4} \cmidrule(r){5-7} \cmidrule(r){8-10} \cmidrule(r){11-13}
& PSNR & SSIM & LPIPS & PSNR & SSIM & LPIPS & PSNR & SSIM & LPIPS & PSNR & SSIM & LPIPS \\
\midrule
4D-GS & 24.29 & \cellcolor{lightyellow}0.9380 & \cellcolor{lightyellow}0.0507 & \cellcolor{lightyellow}38.74 & \cellcolor{lightyellow}0.9535 & \cellcolor{lightyellow}0.0487 & \cellcolor{lightyellow}31.77 & 0.9300 & 0.0485 & \cellcolor{lightyellow}24.29 & \cellcolor{lightyellow}0.9295 & \cellcolor{lightyellow}0.0428 \\
Def-3D-Gauss & \cellcolor{lightred}25.38 & \cellcolor{lightred}0.9790 & \cellcolor{lightred}0.0183 & \cellcolor{lightorange}44.16 & \cellcolor{lightorange}0.9930 & \cellcolor{lightorange}0.0099 & \cellcolor{lightred}38.01 & \cellcolor{lightred}0.9950 & \cellcolor{lightred}0.0063 & \cellcolor{lightred}39.21 & \cellcolor{lightred}0.9895 & \cellcolor{lightred}0.0126 \\
4D-Rotor-Gauss & \cellcolor{lightorange}24.93 & 0.9365 & 0.0541 & 31.77 & 0.9490 & 0.0511 & 30.33 & \cellcolor{lightyellow}0.9430 & \cellcolor{lightyellow}0.0479 & \cellcolor{lightorange}33.40 & 0.9190 & 0.0521 \\
Ours & \cellcolor{lightyellow}24.74 & \cellcolor{lightorange}0.9680 & \cellcolor{lightorange}0.0191 & \cellcolor{lightred}44.66 & \cellcolor{lightred}0.9940 & \cellcolor{lightred}0.0088 & \cellcolor{lightorange}37.24 & \cellcolor{lightorange}0.9730 & \cellcolor{lightorange}0.0162 & 23.93 & \cellcolor{lightorange}0.9700 & \cellcolor{lightorange}0.0129 \\
\bottomrule
\end{tabular}
\caption{Quantitative comparison on D-NeRF dataset with \textbf{black background}. For all metrics, PSNR$\uparrow$, SSIM$\uparrow$ indicate higher is better, while LPIPS$\downarrow$ indicates lower is better. \colorbox{lightred}{Red}, \colorbox{lightorange}{orange}, and \colorbox{lightyellow}{yellow} indicate the best, second-best, and third-best results respectively. We change the default background colors as set in their official released code.}
\label{tab:dnerf_scenes_black}
\end{table*}

\section{Per-Scene Results}

We provide detailed per-scene quantitative comparisons on the D-NeRF dataset to demonstrate the effectiveness of our method across various dynamic scenes. Table~\ref{tab:dnerf_scenes} and ~\ref{tab:dnerf_scenes_black} presents the results for each scene, comparing our method with several state-of-the-art approaches. We provide video demonstrations in the supplementary material, which are rendered from fixed camera viewpoints using interpolated continuous timestamps.

\subsection{Analysis of Results}

Our method demonstrates strong performance across most scenes in terms of PSNR, SSIM, and LPIPS metrics. In the \textit{Hell Warrior} scene, \textit{Def-3D-Gauss} achieves the highest PSNR of \textcolor{red}{41.54}, while our method follows closely with \textcolor{orange}{39.06}. This close performance demonstrates the effectiveness of our Wasserstein-constrained state-space modeling in capturing complex dynamic motions.

In the \textit{Mutant} scene, \textit{Def-3D-Gauss} attains a PSNR of \textcolor{orange}{39.26}, while our method achieves a superior PSNR of \textcolor{red}{40.77}. Our method also demonstrates better perceptual quality with the lowest LPIPS of \textcolor{red}{0.0048}, indicating both higher reconstruction quality and better visual results.

For scenes with rapid motions like \textit{Bouncing Balls} and \textit{Jumping Jacks}, our method maintains robust performance. In \textit{Bouncing Balls}, we achieve a PSNR of \textcolor{red}{42.79}, surpassing \textit{Def-3D-Gauss}'s \textcolor{orange}{41.01}. In \textit{Jumping Jacks}, our method leads with a PSNR of \textcolor{red}{37.91}, showcasing our capability in handling challenging dynamic content. The incorporation of Wasserstein geometry allows for smooth and consistent updates of Gaussian parameters, effectively reducing artifacts and ensuring temporal coherence.

Compared to previous methods like \textit{4D-GS} and \textit{4D-Rotor-Gauss}, our method shows consistent improvements across most scenes. For example, in the \textit{Lego} scene, our method achieves a PSNR of \textcolor{red}{34.74}, surpassing \textit{4D-Rotor-Gauss} by approximately \textcolor{red}{9.5} dB and exceeding \textit{Def-3D-Gauss} by \textcolor{red}{1.67} dB.

Overall, these results indicate that our method achieves superior average performance while maintaining competitive or leading metrics in most scenes. This confirms the effectiveness of integrating Wasserstein geometry and state-space modeling for dynamic scene rendering.

\subsection{Comparison with Baseline Methods}

Compared to methods like \textit{DyNeRF} and \textit{StreamRF}, which primarily rely on Euclidean metrics for parameter updates, our approach offers a more geometrically meaningful way to model Gaussian dynamics. The consistent performance improvements illustrate the advantages of our geometric approach over traditional methods.

Methods like \textit{Def-3D-Gauss} and \textit{4D-Rotor-Gauss} improve upon traditional approaches by considering deformations and rotations, and our method builds upon these advances by incorporating Wasserstein geometry and state-space modeling. This comprehensive framework leads to more robust and consistent results across various dynamic scenes.

% \section{Conclusion}

% By incorporating the numerical stabilization techniques detailed above, we ensure that our computations of the logarithmic and exponential maps in the Wasserstein space are robust and accurate. These measures are crucial for the reliable modeling of Gaussian dynamics in dynamic scene rendering, preventing numerical instabilities that could lead to incorrect results or computational errors.
